# Supplementary material for: Resolving 3D Human Pose Ambiguities with 3D Scene Constraints
Source: arXiv:1908.06963 source file (2019-08-20)
Supplement: Supplementary file 2 [file iccv2019_human_world___SUPPLEMENTARY___00__COMPRESSED.pdf]

# Resolving 3D Human Pose Ambiguities with 3D Scene Constraints

## \*\*Supplementary Material\*\*

Mohamed Hassan, Vasileios Choutas, Dimitrios Tzionas and Michael J. Black

Max Planck Institute for Intelligent Systems

{mhassan, vchoutas, dtzionas, black}@tuebingen.mpg.de

Our method enforces *Proximal Relationships with Object eXclusion* and is called *PROX*. The figures below show representative examples where the human body pose is estimated with (gray color) and without (yellow color) our environmental terms. From the viewpoint of the camera, both solutions look good and match the 2D image features but, when placed in a scan of the 3D scene, the results without environment constraints can be grossly inaccurate. Adding our constraints to the optimization reduces inter-penetration and encourages appropriate contact.

**Why such constraints are not typically used?** One key reason is that to estimate and reason about contact and inter-penetration, one needs *both* a model of the 3D *scene* and a realistic model of the *human body*. The former is easy to obtain today with many scanning technologies but, if the body model is not accurate, it does not make sense to reason about contact and inter-penetration. Consequently we use the SMPL-X body model [3], which is realistic enough to serve as a “proxy” for the real human in the 3D scene. In particular, the feet, hands, and body of the model have realistic shape and degrees of freedom.

**Is it realistic to assume a 3D scene for refining pose?** Here we assume that a rough 3D model of the scene is available; one could argue that this is a hard assumption. Reconstructing a 3D scene from a single RGB image is a hot research topic, but the problem is ill-posed and currently unsolved. Here we want to show in the first place that knowledge about the scene helps pose estimation. Our results support this hypothesis, and scanning a scene today is quite easy. Our next step is to relax this assumption, and move to the more difficult problem of exploiting recent deep networks to estimate the scene directly from monocular RGB images. There are now good methods to infer depth maps from a single image [1] as well as methods that do more semantic analysis and estimate 3D CAD models of the objects in the scene [2]. Our work is complementary to this direction and we believe that monocular 3D scene estimation and monocular 3D human pose estimation should happen together. The work here provides a clear example of why this is valuable.

## Qualitative Results - Our Dataset

Figures A.1-A.3 show additional qualitative results for our method (light gray) on our PROX dataset and compare it to the RGB-only baseline (yellow). For each example we show from left to right: (1) RGB image, (2) renderings from different viewpoints.

## Qualitative Results - PiGraphs

Figure A.4 shows additional qualitative results for our method (light gray) on the *PiGraphs* dataset [4] and compare it to the RGB-only baseline (yellow). Please note that [4] estimate just a 3D skeleton of only the major body joints. In contrast, we estimate a full 3D mesh, and include facial expressions and finger articulation. The mesh representation of our realistic human model helps to better reason about proximity to the world, contact and penetrations. For each example we show from left to right: (1) RGB image, (2) renderings from different viewpoints.

## Computational Complexity

Table A.1 reports the average runtime for all our configurations (PROX in bold) for 10 randomly sampled frames. Compared to using RGB alone; PROX improved “V2V” by 24% with a runtime increase of 41%.

| $E_J$ | $E_P$ | $E_C$ | $E_D$ | Run time     | cos |
|-------|-------|-------|-------|--------------|-----|
| ✓     | ✗     | ✗     | ✗     | 33.75        |     |
| ✓     | ✓     | ✗     | ✗     | 46.91        |     |
| ✓     | ✗     | ✓     | ✗     | 42.68        |     |
| $E_J$ | $E_P$ | $E_C$ | $E_D$ | Run time     | cos |
| ✓     | ✓     | ✓     | ✗     | <b>47.64</b> |     |
| ✓     | ✗     | ✗     | ✓     | 54.28        |     |
| ✓     | ✓     | ✓     | ✓     | 73.08        |     |

Table A.1: Runtime for all configurations of our approach.

## Choice of Contact Vertices

We choose the body vertices that often come in contact with the 3D world. This choice is not exclusive. Table A.2 evaluates different sets of candidate contact vertices, namely our annotations and all vertices. Performance deteriorates in the latter case, while runtime increases by  $\sim 7$  seconds. This suggests the importance of affordances and

semantics; future work can learn the likely contact vertices for different object classes in a data-driven fashion. To this end, the community first needs training data similar to the data generated by our work.

| Contact vertices   | PJE    | V2V    | p.PJE | p.V2V |   |
|--------------------|--------|--------|-------|-------|---|
| Selected of Fig. 2 | 208.03 | 208.57 | 72.76 | 60.95 | m |
| All selected       | 217.82 | 216.62 | 72.35 | 60.16 |   |

Table A.2: Different sets of candidate contact vertices.

## Failure Cases

Figures A.5-A.6 show failure cases of our method (light gray) on our PROX dataset. For each example we show from left to right: (1) RGB image, (2) OpenPose result overlaid on the RGB image, (3) result of our method. Figure A.5-top shows that our method still results in some penetration. Our assumption of a static scene is not always true; in this case the bed is deformable and its shape changes during interaction. In future work we plan to model deformations of the human body and the world. Figure A.5-bottom shows a failure of our inter-penetration term. In cases where initialization of body translation is not accurate enough, the optimizer might end up in a local minimum that is not always in agreement with the real pose in 3D space. Figure A.6 shows typical failure cases of OpenPose. In Figure A.6-top the left leg is not detected correctly, while in Figure A.6-middle and Figure A.6-bottom several body joints are flipped by OpenPose.

## References

- [1] David Eigen, Christian Puhrsch, and Rob Fergus. Depth map prediction from a single image using a multi-scale deep network. In *Advances in Neural Information Processing Systems*, pages 2366–2374, 2014. 1
- [2] Muzammal Naseer, Salman Khan, and Fatih Porikli. Indoor scene understanding in 2.5/3d for autonomous agents: A survey. *IEEE Access*, 7:1859–1887, 2019. 1
- [3] Georgios Pavlakos, Vasileios Choutas, Nima Ghorbani, Timo Bolkart, Ahmed A. A. Osman, Dimitrios Tzionas, and Michael J. Black. Expressive body capture: 3d hands, face, and body from a single image. In *The IEEE Conference on Computer Vision and Pattern Recognition (CVPR)*, 2019. 1
- [4] Manolis Savva, Angel X Chang, Pat Hanrahan, Matthew Fisher, and Matthias Nießner. Pigraphs: learning interaction snapshots from observations. *ACM Transactions on Graphics (TOG)*, 35(4):139, 2016. 1, 6

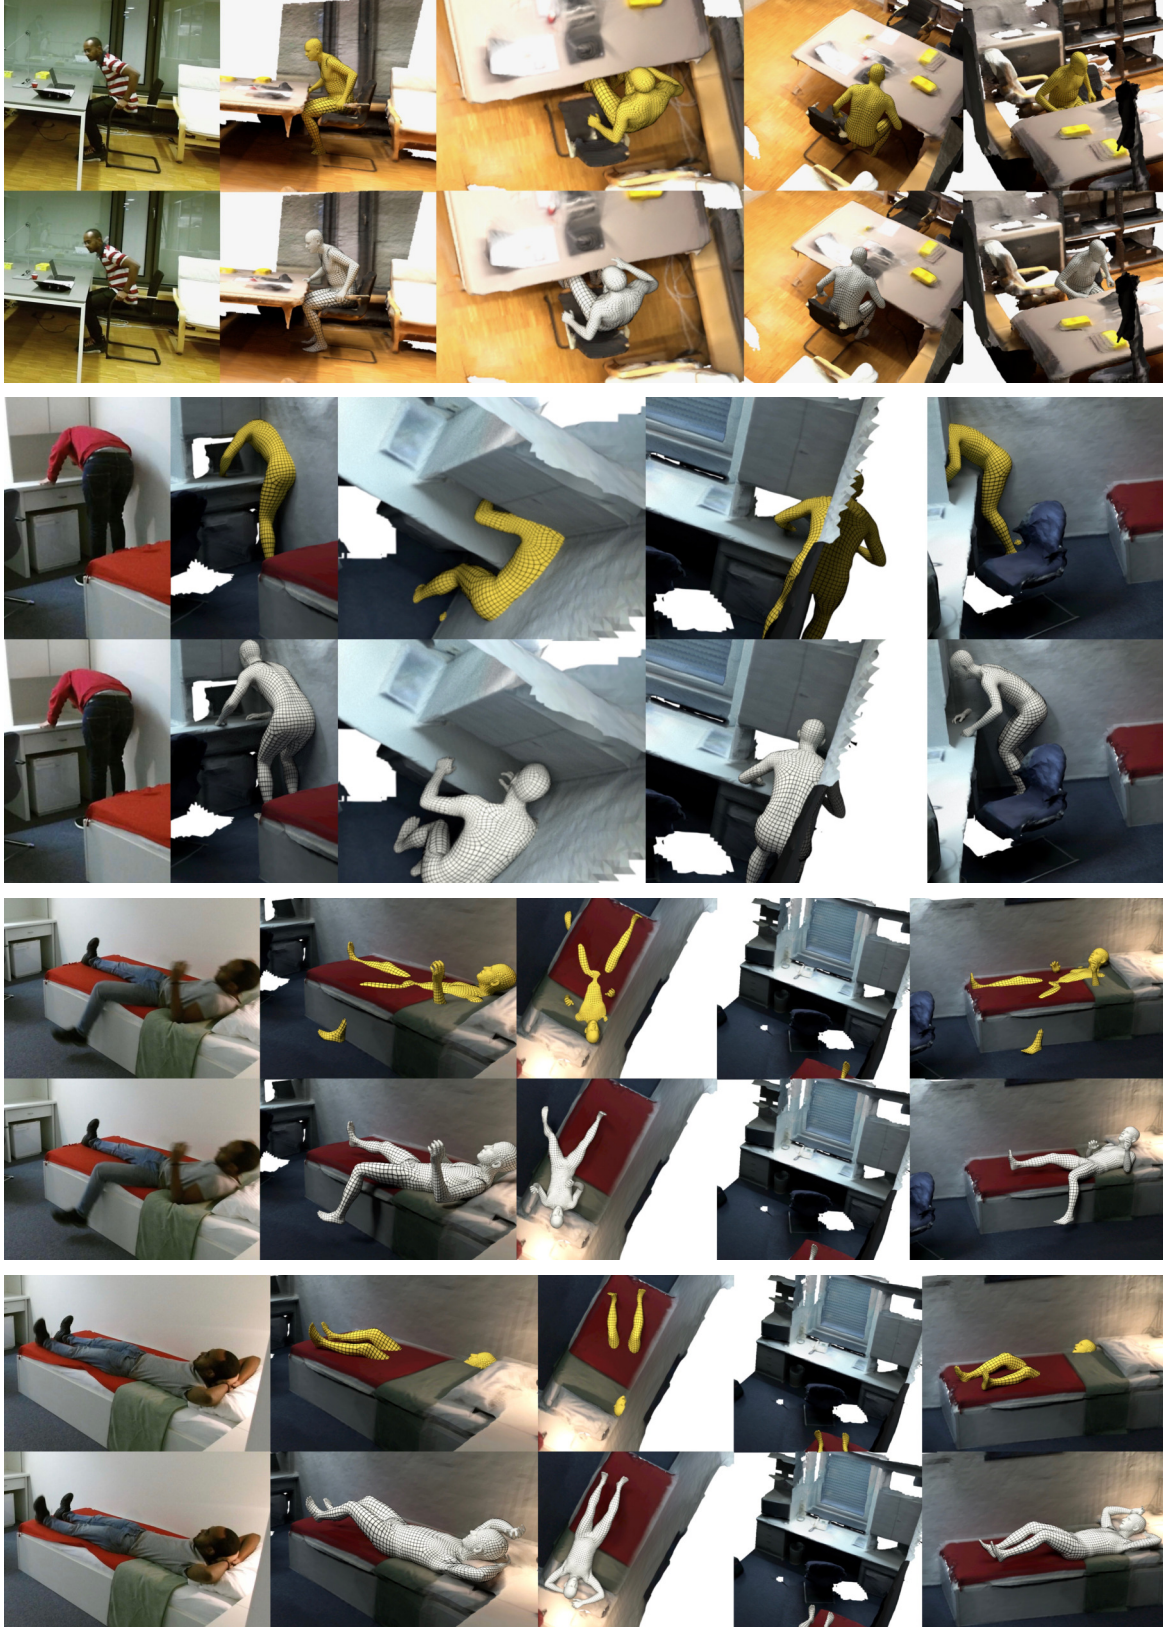

Figure A.1: Qualitative results on our PROX dataset. The human body pose is estimated *with* (light gray) and *without* (yellow) our environmental terms. We show from left to right: (1) RGB images, (2) renderings from different viewpoints.



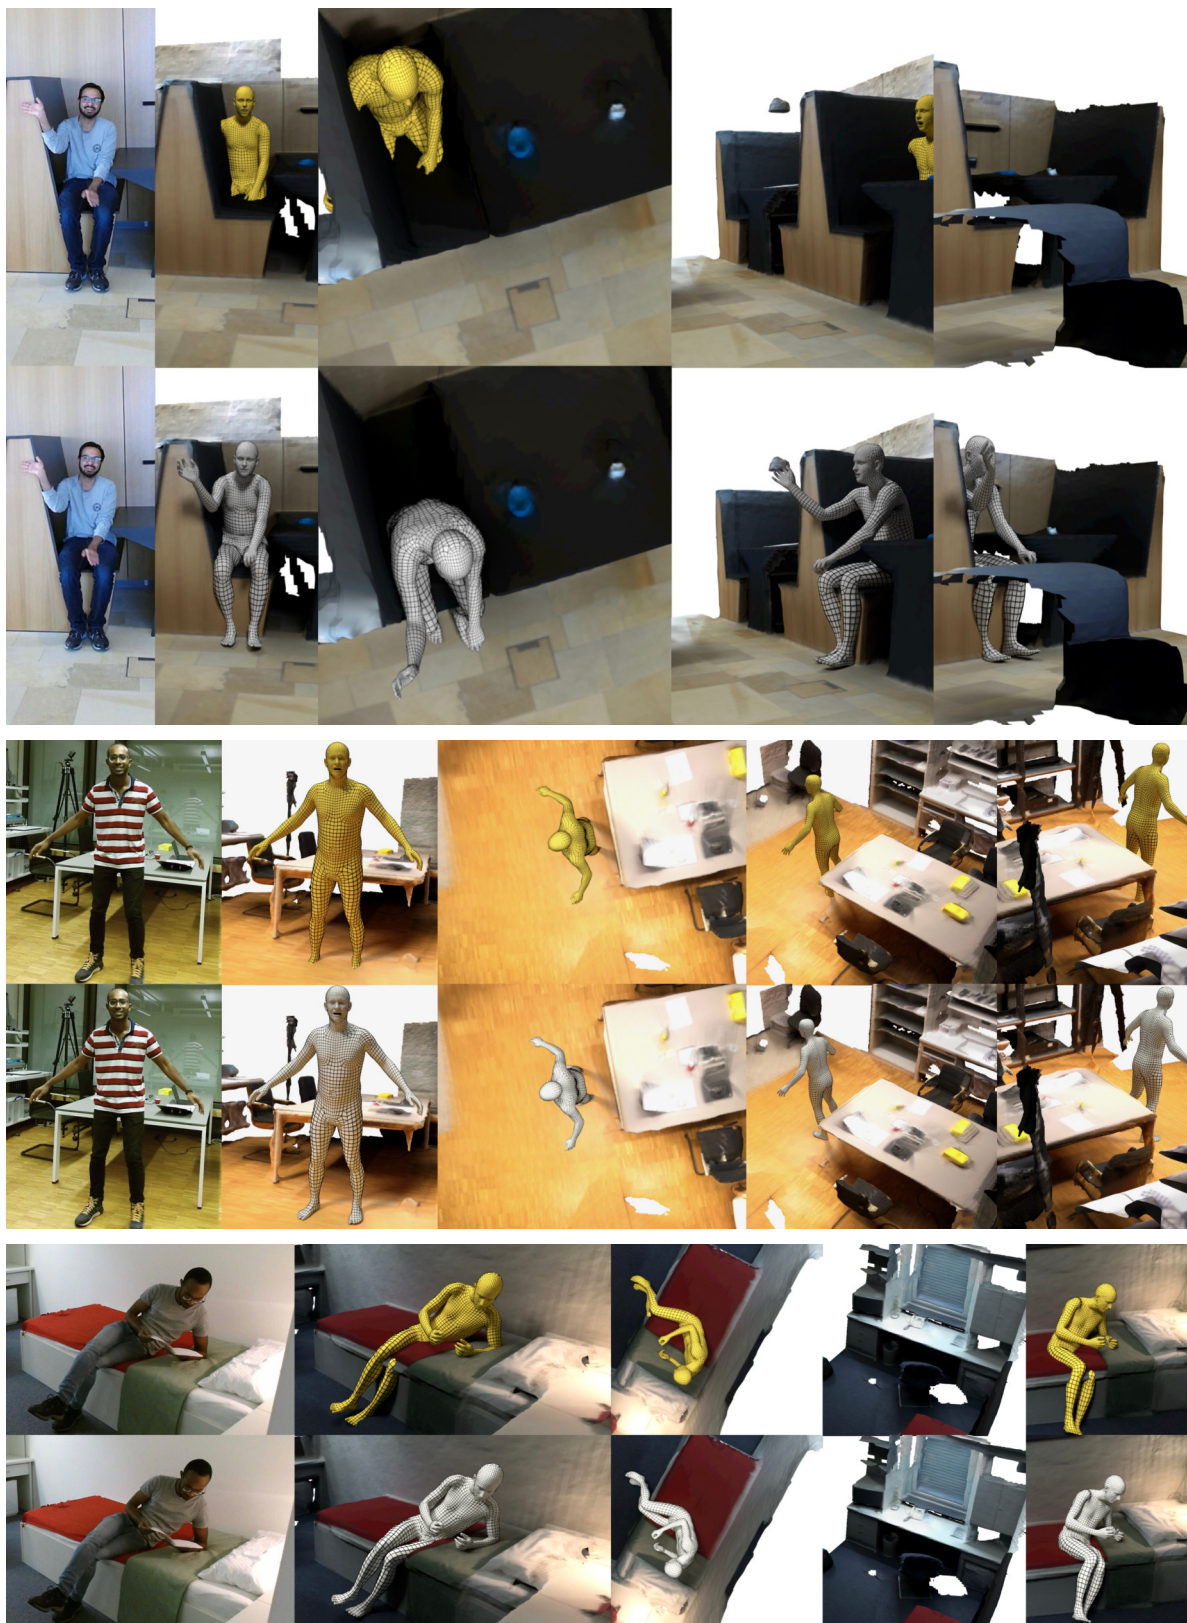

Figure A.2: Qualitative results on our PROX dataset. The human body pose is estimated *with* (light gray) and *without* (yellow) our environmental terms. We show from left to right: (1) RGB images, (2) renderings from different viewpoints.



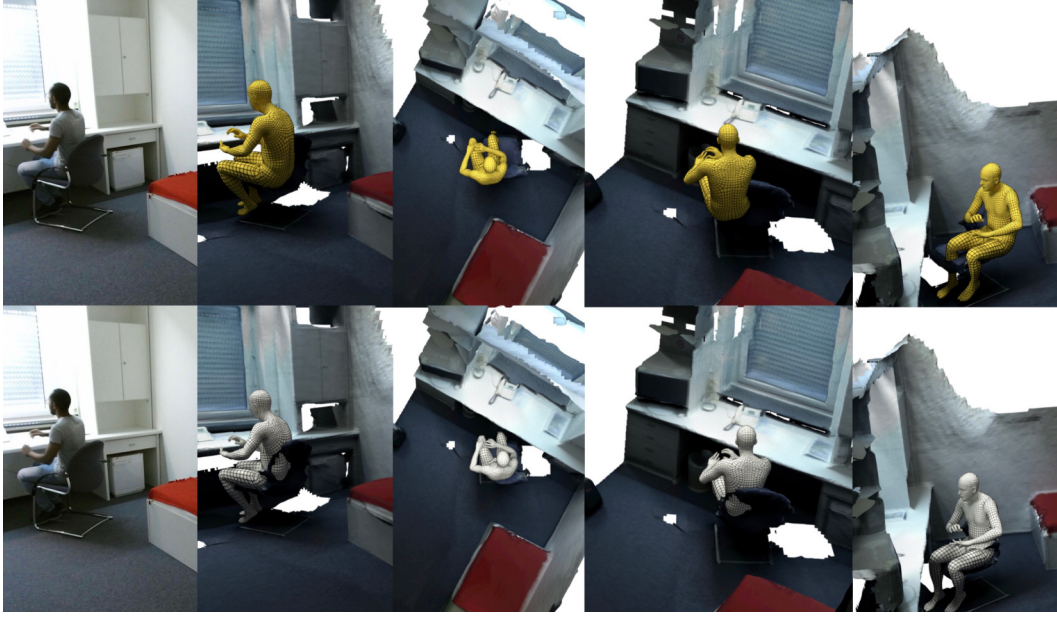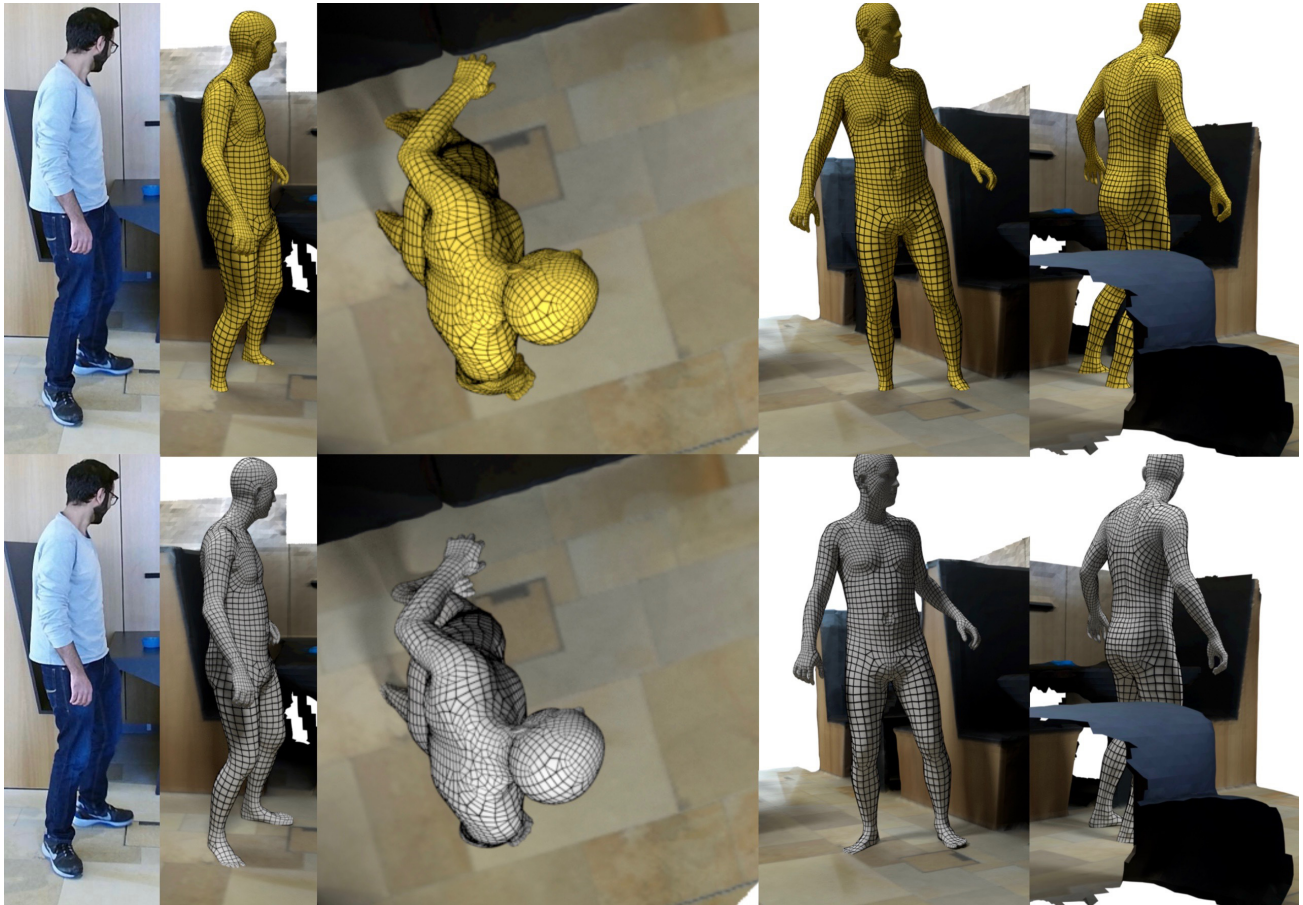

Figure A.3: Qualitative results on our PROX dataset. The human body pose is estimated *with* (light gray) and *without* (yellow) our environmental terms. We show from left to right: (1) RGB images, (2) renderings from different viewpoints.



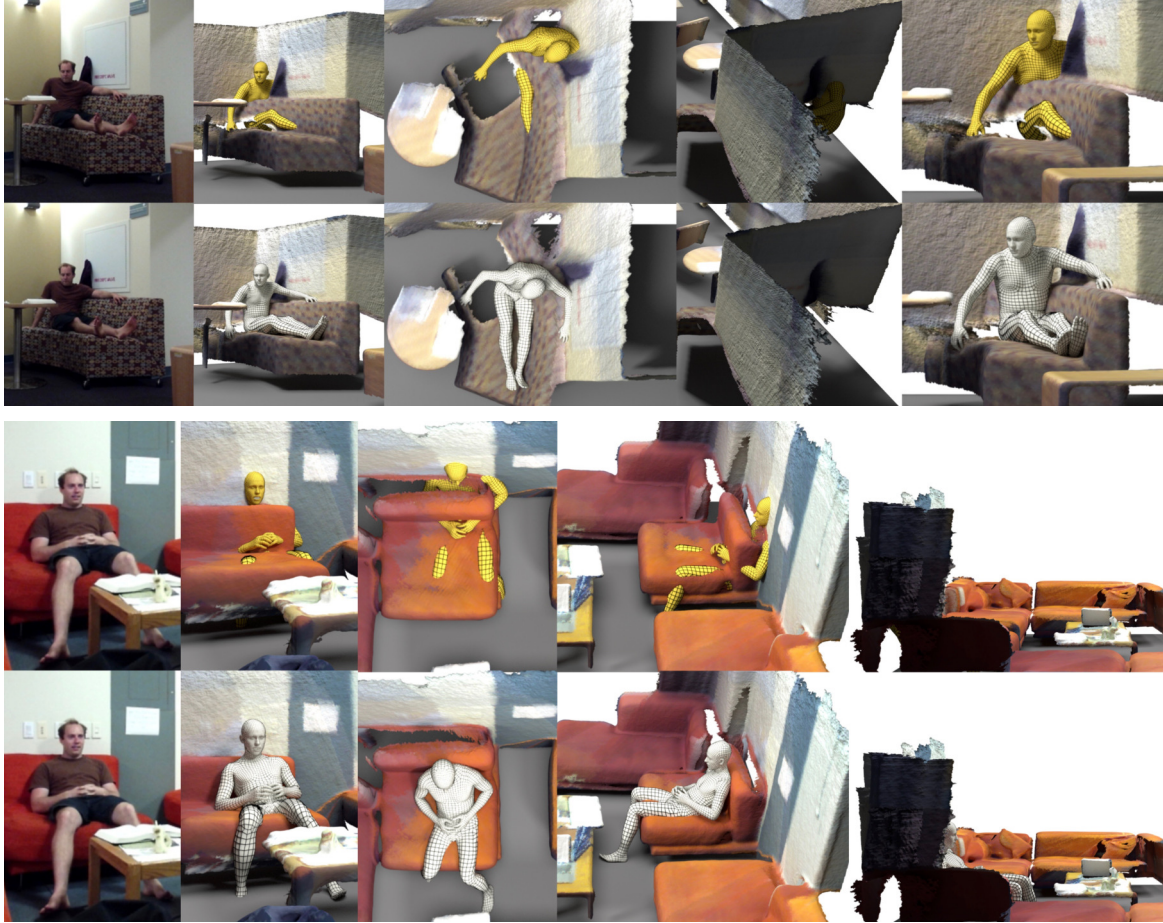

Figure A.4: Qualitative results on the PiGraphs [4] dataset. The human body pose is estimated *with* (gray color) and *without* (yellow color) our environmental terms. Please note that [4] estimate just a 3D skeleton of only the major body joints. We show from left to right: (1) RGB images, (2) renderings from different viewpoints.

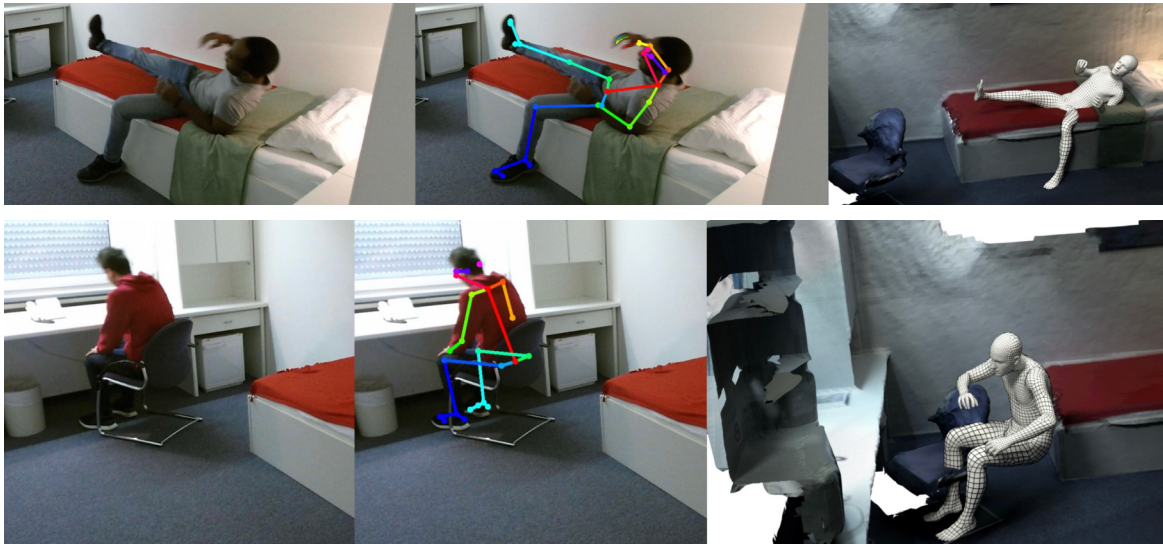

Figure A.5: Representative failure cases on our PROX dataset. We show from left to right: (1) RGB image, (2) OpenPose result overlaid on the RGB image, (3) result of our method.



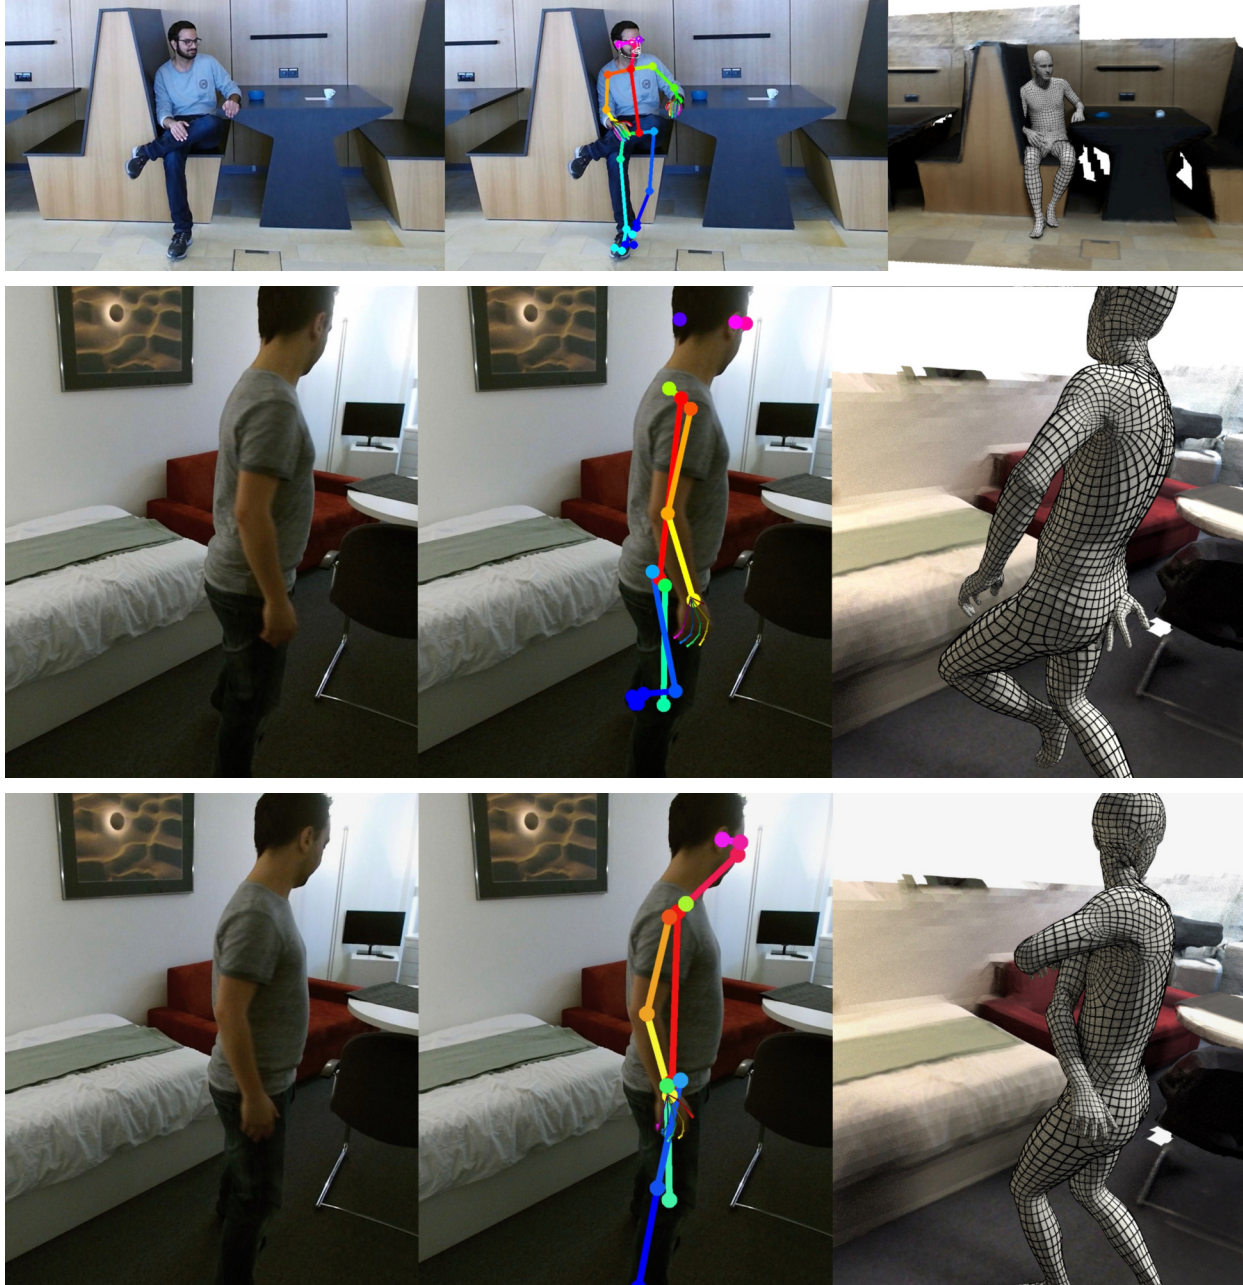

Figure A.6: Representative failure cases on our PROX dataset. We show from left to right: (1) RGB image, (2) OpenPose result overlaid on the RGB image, (3) result of our method.
